# Supplementary material for: A Simple Explanation for the Observed Power Law Distribution of Line Intensity in Complex Many-Electron Atoms
Source: arXiv:1908.10464 source file (2020-04-14)
Supplement: Supplementary file 1 [file main_supplemental.tex]

\documentclass[%
 reprint,
%superscriptaddress,
%groupedaddress,
%unsortedaddress,
%runinaddress,
%frontmatterverbose,
%preprint,
%preprintnumbers,
%nofootinbib,
%nobibnotes,
%bibnotes,
 amsmath,amssymb,
 aps,
%pra,
%prb,
%rmp,
%prstab,
%prstper,
%floatfix,
]{revtex4-1}

\usepackage{graphicx}% Include figure files

\begin{document}
\input{supplemental.tex}

\bibliography{../refs} % Produces the bibliography via BibTeX.
\end{document}
